# Supplementary material for: Observability Analysis of Aided INS with Heterogeneous Features of Points, Lines and Planes
Source: arXiv:1805.05876 source file (2018-05-12)
Supplement: Supplementary file 1 [file momo_point.tex]

%!TEX root = ../main.tex

\section{Bearing Measurements of Points for a Monocular Camera} \label{apd_mono_bearing}
%todo: make a small change of the bearing measurement equations
%todo: change {}^Iz_{\mathbf{f}}}  to \mathbf{e}^{\top}_3 {^I\mathbf{P}_{\mathbf{f}}}
Geometrically, a monocular camera  provide only bearing information of a point feature, 
whose bearing measurement model is given by:
\begin{equation}\label{eq_mono_cam}
\mathbf{z}^{(b)}  
= 
\begin{bmatrix}
\frac{\mathbf{e}_1^{\top}{^I\mathbf{P}_{\mathbf{f}}}}{\mathbf{e}_3^{\top}{^I\mathbf{P}_{\mathbf{f}}}} \\
\frac{\mathbf{e}_2^{\top}{^I\mathbf{P}_{\mathbf{f}}}}{\mathbf{e}_3^{\top}{^I\mathbf{P}_{\mathbf{f}}}} 
\end{bmatrix} 
+ \mathbf{n}^{(b)}
= 
\begin{bmatrix}
\frac{^Ix_{\mathbf{f}}}{^Iz_{\mathbf{f}}}  \\
\frac{^Iy_{\mathbf{f}}}{^Iz_{\mathbf{f}}}
\end{bmatrix}  
+ \mathbf{n}^{(b)}
\end{equation}
where 
$\mathbf{e}_i\in \mathbb{R}^{3\times1}$ ($i=1,2,3$) are the canonical  basis unit vectors, i.e., 
$\mathbf{e}_1=[1\quad0\quad0]^{\top}$, $\mathbf{e}_2=[0\quad1\quad0]^{\top}$ and $\mathbf{e}_3=[0\quad0\quad1]^{\top}$. 
As in our prior work~\cite{Yang2017SSRR}, we use the following bearing measurement model for a point feature:
\begin{align}\label{eq_mono_meas}
	\mathbf{z}^{(b)} &=
	\mathbf{h}_{b}\left({^I\mathbf{P}_{\mathbf{f}}}, {\mathbf{n}^{(b)}}\right)
	\nonumber
	\\
	&=
	\begin{bmatrix}
	^I\mathbf{b}^{\top}_{\perp1} \\
	^I\mathbf{b}^{\top}_{\perp2} 
	\end{bmatrix}
	{^I\mathbf{P}_{\mathbf{f}}}
	+
	%{^Iz_{\mathbf{f}}}
	\mathbf{e}^{\top}_3 {^I\mathbf{P}_{\mathbf{f}}}
	\begin{bmatrix}
	^I\mathbf{b}^{\top}_{\perp1} \\
	^I\mathbf{b}^{\top}_{\perp2} 
	\end{bmatrix}
	\begin{bmatrix}
	\mathbf{I}_2 \\
	\mathbf{0}_{1\times 2}
	\end{bmatrix}
	\mathbf{n}^{(b)}
\end{align}
where $^I\mathbf{b}_{\perp i},i\in\{1,2\}$ are two orthogonal vectors to the bearing vector 
$^I\mathbf{b}_{\mathbf f}$, and  can be easily constructed as in~\cite{Yang2017SSRR}. 
%The advantage of this model is that it is suitable for both fish eye and normal projective camera model. 
To obtain the Jacobians, we linearize the model about the current estimate of feature-to-camera relative position $^I\hat{\mathbf{P}}_{\mathbf{f}}$ as follows:
\begin{align}\label{eq_mono_meas_linear}
	\tilde{\mathbf{z}}^{(b)}
	&\simeq
	\mathbf{H}_{b}{^I\tilde{\mathbf{P}}_{\mathbf{f}}} +
	\mathbf{H}_{n}\mathbf{n}^{(b)}
	\nonumber
	\\
	&=
	\begin{bmatrix}
	^I\hat{\mathbf{b}}^{\top}_{\perp1} \\
	^I\hat{\mathbf{b}}^{\top}_{\perp2} 
	\end{bmatrix}
	{^I\tilde{\mathbf{P}}_{\mathbf{f}}}
	+
	%{^I\hat{z}_{\mathbf{f}}}
	\mathbf{e}^{\top}_3 {^I\hat{\mathbf{P}}_{\mathbf{f}}}
	\begin{bmatrix}
	^I\hat{\mathbf{b}}^{\top}_{\perp1} \\
	^I\hat{\mathbf{b}}^{\top}_{\perp2} 
	\end{bmatrix}
	\begin{bmatrix}
	\mathbf{I}_2 \\
	\mathbf{0}_{1\times 2}
	\end{bmatrix}
	\mathbf{n}^{(b)}
\end{align}
